# Supplementary material for: Measurement of the Coherent Elastic Neutrino-Nucleus Scattering Cross Section on CsI by COHERENT
Source: arXiv:2110.07730 ancillary file (2022-06-02)
Supplement: Supplementary file 1 [file Paper_CEvNSCsI_FullDataset_SupMaterials.pdf]

# Supplemental Material: Measurement of the Coherent Elastic Neutrino-Nucleus Scattering Cross Section on CsI by COHERENT

D. Akimov,<sup>1</sup> P. An,<sup>2,3</sup> C. Awe,<sup>2,3</sup> P.S. Barbeau,<sup>2,3</sup> B. Becker,<sup>4</sup> V. Belov,<sup>5,1</sup> I. Bernardi,<sup>4</sup> M.A. Blackston,<sup>6</sup> C. Bock,<sup>7</sup> A. Bolozdynya,<sup>1</sup> J. Browning,<sup>8</sup> B. Cabrera-Palmer,<sup>9</sup> D. Chernyak,<sup>7,\*</sup> E. Conley,<sup>2</sup> J. Daughhetee,<sup>6</sup> J. Detwiler,<sup>10</sup> K. Ding,<sup>7</sup> M.R. Durand,<sup>10</sup> Y. Efremenko,<sup>4,6</sup> S.R. Elliott,<sup>11</sup> L. Fabris,<sup>6</sup> M. Febraro,<sup>6</sup> A. Gallo Rosso,<sup>12</sup> A. Galindo-Uribarri,<sup>6,4</sup> M.P. Green,<sup>3,6,8</sup> M.R. Heath,<sup>6</sup> S. Hedges,<sup>2,3</sup> D. Hoang,<sup>13</sup> M. Hughes,<sup>14</sup> T. Johnson,<sup>2,3</sup> A. Khromov,<sup>1</sup> A. Konovalov,<sup>1,5</sup> E. Kozlova,<sup>1,5</sup> A. Kumpan,<sup>1</sup> L. Li,<sup>2,3</sup> J.M. Link,<sup>15</sup> J. Liu,<sup>7</sup> K. Mann,<sup>8</sup> D.M. Markoff,<sup>16,3</sup> J. Mastroberti,<sup>14</sup> P.E. Mueller,<sup>6</sup> J. Newby,<sup>6</sup> D.S. Parno,<sup>13</sup> S.I. Penttila,<sup>6</sup> D. Pershey,<sup>2</sup> R. Rapp,<sup>13</sup> H. Ray,<sup>17</sup> J. Raybern,<sup>2</sup> O. Razuvaeva,<sup>1,5</sup> D. Reyna,<sup>9</sup> G.C. Rich,<sup>3</sup> J. Ross,<sup>16,3</sup> D. Rudik,<sup>1</sup> J. Runge,<sup>2,3</sup> D.J. Salvat,<sup>14</sup> A.M. Salyapongse,<sup>13</sup> K. Scholberg,<sup>2</sup> A. Shakirov,<sup>1</sup> G. Simakov,<sup>1,5</sup> G. Sinev,<sup>2,†</sup> W.M. Snow,<sup>14</sup> V. Sosnovstsev,<sup>1</sup> B. Suh,<sup>14</sup> R. Tayloe,<sup>14</sup> K. Tellez-Giron-Flores,<sup>15</sup> I. Tolstukhin,<sup>14,‡</sup> E. Ujah,<sup>16,3</sup> J. Vanderwerp,<sup>14</sup> R.L. Varner,<sup>6</sup> C.J. Virtue,<sup>12</sup> G. Visser,<sup>14</sup> T. Wongjirad,<sup>18</sup> Y.-R. Yen,<sup>13</sup> J. Yoo,<sup>19</sup> C.-H. Yu,<sup>6</sup> and J. Zettlemoyer<sup>14,§</sup>

<sup>1</sup>National Research Nuclear University MEPhI (Moscow Engineering Physics Institute), Moscow, 115409, Russian Federation

<sup>2</sup>Department of Physics, Duke University, Durham, NC, 27708, USA

<sup>3</sup>Triangle Universities Nuclear Laboratory, Durham, NC, 27708, USA

<sup>4</sup>Department of Physics and Astronomy, University of Tennessee, Knoxville, TN, 37996, USA

<sup>5</sup>Institute for Theoretical and Experimental Physics named by A.I. Alikhanov of National Research Centre “Kurchatov Institute”, Moscow, 117218, Russian Federation

<sup>6</sup>Oak Ridge National Laboratory, Oak Ridge, TN, 37831, USA

<sup>7</sup>Physics Department, University of South Dakota, Vermillion, SD, 57069, USA

<sup>8</sup>Department of Physics, North Carolina State University, Raleigh, NC, 27695, USA

<sup>9</sup>Sandia National Laboratories, Livermore, CA, 94550, USA

<sup>10</sup>Center for Experimental Nuclear Physics and Astrophysics & Department of Physics, University of Washington, Seattle, WA, 98195, USA

<sup>11</sup>Los Alamos National Laboratory, Los Alamos, NM, 87545, USA

<sup>12</sup>Department of Physics, Laurentian University, Sudbury, Ontario, P3E 2C6, Canada

<sup>13</sup>Department of Physics, Carnegie Mellon University, Pittsburgh, PA, 15213, USA

<sup>14</sup>Department of Physics, Indiana University, Bloomington, IN, 47405, USA

<sup>15</sup>Center for Neutrino Physics, Virginia Tech, Blacksburg, VA, 24061, USA

<sup>16</sup>Department of Mathematics and Physics, North Carolina Central University, Durham, NC, 27707, USA

<sup>17</sup>Department of Physics, University of Florida, Gainesville, FL, 32611, USA

<sup>18</sup>Department of Physics and Astronomy, Tufts University, Medford, MA, 02155, USA

<sup>19</sup>Department of Physics and Astronomy, Seoul National University, Seoul, 08826, Korea

With this supplemental material, we provide selected, unbinned data events relevant for this result. Candidate waveforms are triggered from the accelerator, pulsed at 60 Hz with a FWHM of 378 ns. A sample waveform is shown in Fig. 1 illustrating epochs in our waveform analysis. There are two regions of interest: beam coincident (C) which encapsulates all beam-related activity and beam anti-coincident (AC) which immediately precedes the arrival of the beam. Each region of interest has a 40  $\mu$ s pretrace used to estimate the background scintillation activity in the crystal on a spill-by-spill basis. Reconstructed events have a 3  $\mu$ s integration window. For each event, we reconstruct and observed energy in photoelectrons (PE) and recoil time,  $t_{\text{rec}}$ .

We also provide signal parameters, neutron background distributions, and details of systematic uncertainty to allow for future study of this analysis sample. All events selected with  $\text{PE} < 250$  and  $0 \leq t_{\text{rec}} < 12 \mu\text{s}$  are included. Events with energy  $60 \leq \text{PE} < 250$  or  $t_{\text{rec}} \geq 6 \mu\text{s}$  are not used for measuring the CEvNS cross section but used for a search for light dark matter produced at the SNS.

\* Now at: Institute for Nuclear Research of NASU, Kyiv, 03028, Ukraine

† Now at: South Dakota School of Mines and Technology, Rapid City, SD, 57701, USA

‡ Now at: Argonne National Laboratory, Argonne, IL, 60439, USA

§ Now at: Fermi National Accelerator Laboratory, Batavia, IL, 60510, USA

*Observed data:* Selected events in both the coincidence (C) and anticoincidence (AC) region for beam-on running are given in

- dataBeamOnAC.txt
- dataBeamOnC.txt.

each with reconstructed energy,  $E_{\text{rec}}$ , and recoil time,  $t_{\text{rec}}$ . A comparison of C and AC data is shown in Fig. 2 with a clearly visible beam excess. These two files contain all data relevant for this measurement. The requisite details to produce accurate predictions for signal and background distributions are below.

*Steady-state background:* The beam-uncorrelated, steady-state background (SSBkg) can be estimated from the AC data. For selected events, there is no correlation between  $E_{\text{rec}}$  and  $t_{\text{rec}}$ , and thus the  $E_{\text{rec}}$  distribution can be determined using all selected events. The time distribution is exponential with a decay constant

- $k = -(0.0494 \pm 0.0061)/\mu\text{s}$

determined by fitting the timing distribution of AC events.

*Neutron backgrounds:* We include both prompt beam-related neutron (BRN) and neutrino-induced neutron (NIN) events. The reconstructed energy and time are uncorrelated, and so we include the one-dimensional projections in PE and  $t_{\text{rec}}$ . For each, we provide the timing distribution in  $0.01 \mu\text{s}$  bins normalized to the beam exposure, 13.99 GWhr. We include the prediction for times  $-0.25 \leq t_{\text{rec}} < 6.25 \mu\text{s}$ , to accommodate uncertainty in beam timing. Due to this uncertainty in timing, the time dependent efficiency,  $\varepsilon_T$ , is not applied. This can be included as

$$\varepsilon_T(t_{\text{rec}}) = \begin{cases} 1 & t_{\text{rec}} < a \\ e^{-b(t_{\text{rec}}-a)} & t_{\text{rec}} \geq a \end{cases} \quad (1)$$

with

- $a = 0.52 \mu\text{s}$
- $b = 0.0494 / \mu\text{s}$ .

The smeared PE probability distribution with the energy dependent efficiency,  $\varepsilon_{\text{PE}}$ , applied is included with 1 PE binning. All energy shape uncertainties in both backgrounds have a negligible impact and are not included. These distributions are included as text files:

- brnPE.txt
- brnTrec.txt
- ninPE.txt
- ninTrec.txt.

*Predicting CEvNS signal:* We analyze beam triggers from 13.99 GWhr of accumulated exposure. The neutrino flux through the detector and rate of CEvNS scatters can be calculated with the parameters:

- POT:  $3.198 \times 10^{23}$
- $\nu$  yield:  $0.0848 \pm 10\% \nu/\text{flavor}/p$
- Detector baseline 19.3 m
- Detector mass: 14.6 kg.

The 2D distribution of the neutrino flux at the SNS is given in

- snsFlux2D.root

with a ROOT histogram for each flavor in the flux.

To accurately predict the event totals in the detector as a function of  $E_{\text{rec}}$  and  $t_{\text{rec}}$ , quenching, energy smearing, and detection efficiency must be applied.

Quenching is applied by evaluating the scintillation response curve, empirically parameterized as

$$E_{ee} = f(E_{nr}) = aE_{nr} + bE_{nr}^2 + cE_{nr}^3 + dE_{nr}^4. \quad (2)$$

The best-fit coefficients are provided in

• scintRespCoefficients.txt.

The file also includes coefficients for each of the two quenching uncertainties included, evaluated at  $\pm 1\sigma$  excursions. The light yield for quenched recoils is given by

• Light yield: 13.35 PE/keV<sub>ee</sub>

whose uncertainty has a negligible impact.

Our energy resolution is dominated by photon counting. However, the distribution of SPE charge is broad,  $\mu/\sigma \approx 0.5$ . We thus also incorporated variations in SPE pulse integral on a pulse-by-pulse basis into our energy resolution. Combining these two effects, the smearing was modeled with a gamma function

$$P(x) = \frac{(a(1+b))^{1+b}}{\Gamma(1+b)} x^b e^{-a(1+b)x} \quad (3)$$

where  $x$  is the experimentally observed recoil energy in PE and  $a$  and  $b$  are parameters which depend on the true quenched energy deposition,  $E_{ee}$ , in units of keV<sub>ee</sub>. Empirically, this function fits well to simulated recoil distributions using  $a = 0.0749/E_{ee}$  and  $b = 9.56 \times E_{ee}$  which appropriately models the asymmetric simulated distribution much better than a Gaussian model. Our analysis of the CEvNS cross section made sure to not include energy bins much narrower than the energy resolution. It is essential for any study using finer bins or an unbinned fit to include smearing effects.

Finally, efficiency must also be applied.

$$\varepsilon(\text{PE}, t_{\text{rec}}) = \varepsilon_E(\text{PE}) \times \varepsilon_T(t_{\text{rec}}) \quad (4)$$

which contains uncorrelated factors from the measured  $E_{\text{rec}}$  and  $t_{\text{rec}}$ . We parameterize  $\varepsilon_E$  as

$$\varepsilon_E(x) = \frac{a}{1 + e^{-b(x-c)}} + d \quad (5)$$

where  $x$  is the observed recoil energy in PE and the function is restricted to evaluate at  $\geq 0$ . The relevant coefficients in the best fit scenario and are included in

• effCoefficients.txt

along with coefficients evaluated at  $\pm 1\sigma$  excursions for the uncertainty in the CEvNS efficiency. This efficiency curve and uncertainty band are shown in Fig. 3. The time dependence is given in Eqn. 1.

*Likelihood fit results:* We reject the no-CEvNS hypothesis at 11.6  $\sigma$  level using a profiled log-likelihood fit. Tests were performed to validate the coverage of this fit, and the likelihood curve is shown in Fig. 4 compared to the standard-model prediction. Best-fit pulls on systematic uncertainties were small except in the case of the threshold uncertainty which pulled at 0.4  $\sigma$ . The best-fit values along with 1  $\sigma$  ranges are shown in Table I. Background normalizations agree with our pre-fit assumptions on each component and the CEvNS rate is consistent with the standard model to 1  $\sigma$ .

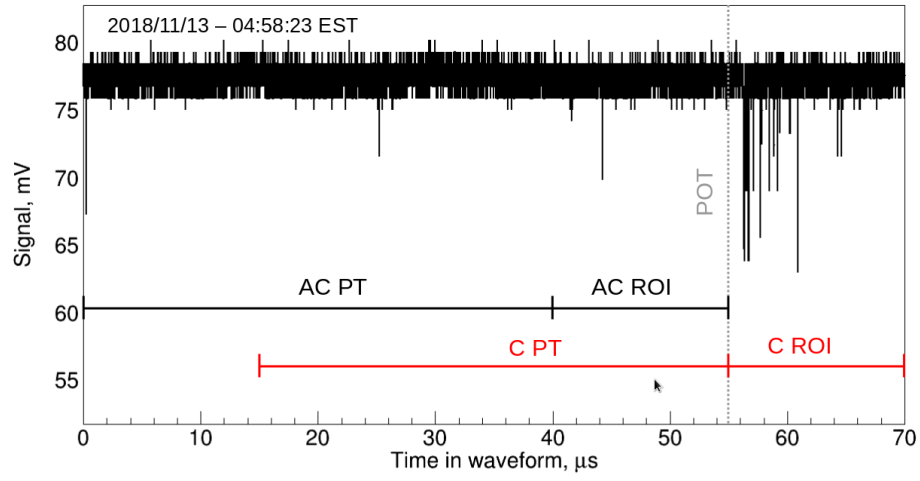

Figure 1. Timing regions of our CsI waveform reconstruction. Events were reconstructed in the 15  $\mu\text{s}$ -long C and AC ROI periods. From the first PE peak in the ROI, we formed a 3  $\mu\text{s}$  integration window. Before each ROI, there is a 40  $\mu\text{s}$ -long pretrace to monitor the instantaneous afterglow rate. The beam arrives at 55  $\mu\text{s}$ , at the beginning of C ROI.

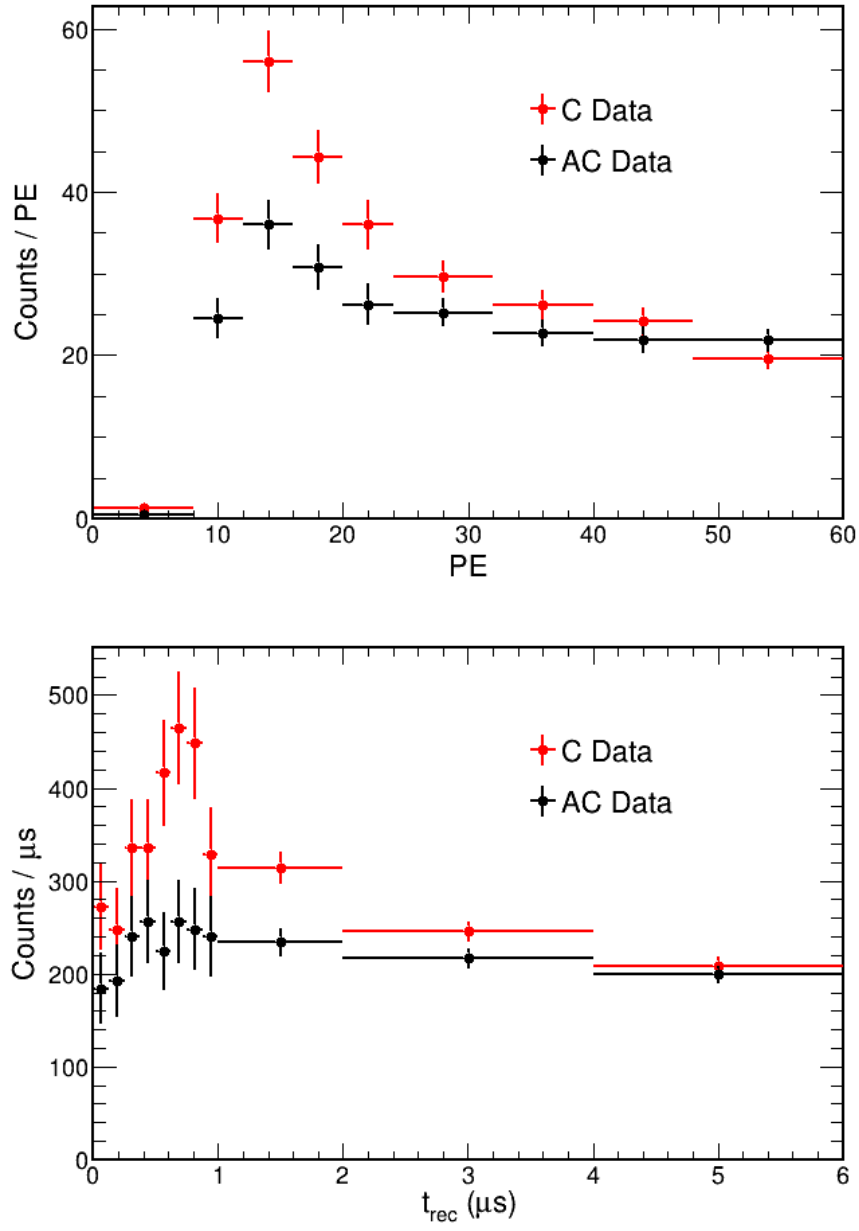

Figure 2. Data after selection with  $t_{\text{rec}} < 6 \mu\text{s}$  collected during SNS operations comparing C and AC ROI data.

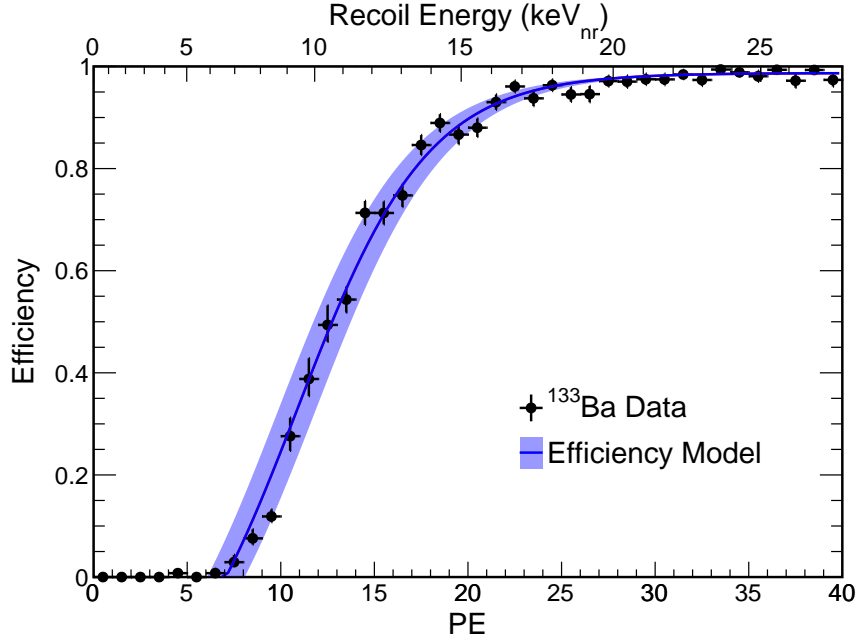

Figure 3. Calibration data using a  $^{133}\text{Ba}$  source to estimate our CEvNS selection efficiency along with an error band.

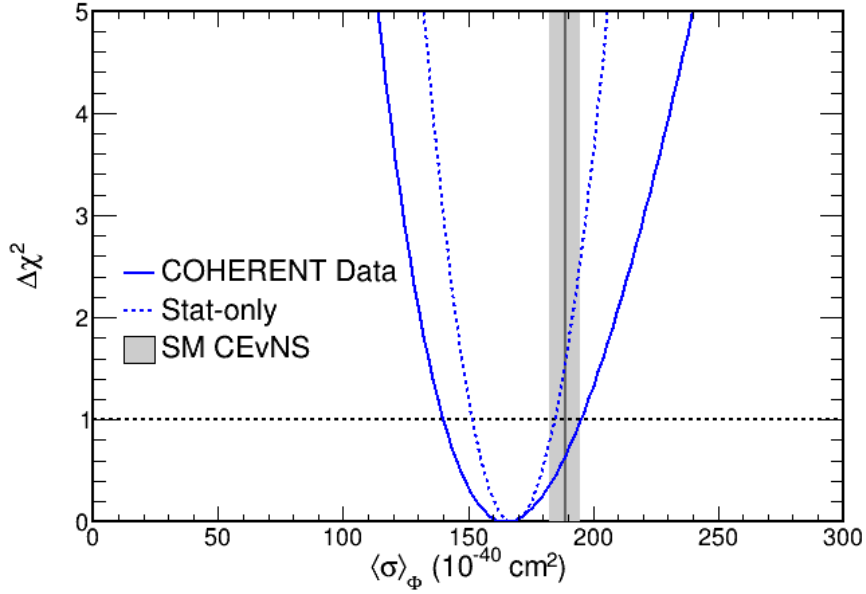

Figure 4. The  $\Delta\chi^2$  curve for the CEvNS cross section determined from the fit to data both with and without systematic effects. The standard-model prediction, along with the  $1\sigma$  error band from the form factor uncertainty is given by the vertical grey band.

|                  | Prior Prediction | Best-Fit Total |
|------------------|------------------|----------------|
| SSBkg background | $1286 \pm 27$    | $1273 \pm 24$  |
| BRN              | $18.4 \pm 4.6$   | $17.3 \pm 4.5$ |
| NIN              | $5.6 \pm 2.0$    | $5.5 \pm 2.0$  |
| CEvNS            | —                | $306 \pm 20$   |

Table I. A summary of prior prediction and best-fit event rates and statistical uncertainties for CEvNS and each background type. The standard-model expectation for CEvNS is  $341 \pm 11 \pm 42$ .
